# Supplementary material for: Representation Learning for Point Cloud Understanding
Source: arXiv:2512.06058 source file (2025-12-05)
Supplement: Supplementary file 1 [file 07_supp.tex]

%We also try a random cropping strategy instead of cropping the center part. During training, we randomly set the cropping location and we hope the model can detect the missing part successfully. The result shows that it is slightly worse than the center cropping. We think that might because our model is not strong enough to fit this strategy. We show more details in supplementary material.
\setcounter{equation}{8}
\setcounter{figure}{5}

%\section{Supplementary Materials}
Our supplementary material provides additional implementation details on scene data generation and pre-training in Section \ref{sec:supp:implement}, more experiment results and analysis in Section \ref{sec:supp:result}, and a theoretical analysis of IAE under a simplified linear
AE model in Section \ref{Section:Motivation}.

\section{Implementation Details}
\label{sec:supp:implement}
\subsection{Scene Data Generation}
Given a point cloud $\mathcal{P}^{\text{gt}}$, we first randomly choose a removing ratio from 0\% to 50\% and apply a center-cropping on it to get the input point cloud  $\mathcal{P}^{\text{in}}$. 
To build the ground truth label of the implicit function $g_0$(e.g., unsigned distance function), we directly compute the distance $d$ between the query point and nearest point from $\mathcal{P}^{\text{gt}}$. And because the point cloud from the real dataset is usually incomplete, we do not define the sign distance values. 
%For the occupancy value, we set the label to be 1 if the distance $d < 0.005m$, and 0 if $d \geq 0.005m$. 

\subsection{Pre-training}
We implement all models in PyTorch and use Adam optimizer with no weight decay. The learning rate is set to $10^{-4}$ for all datasets. For ShapeNet, we pre-train the models for 600 epochs. And for ScanNet, we pre-train the models for 1000 epochs.

\section{More Results}
\label{sec:supp:result}

\subsection{Label Efficiency Training}
Pretraining helps models to be fine-tuned with small amount of labeled data. We study the label efficiency of our model on 3D object detection by varying the portion of supervised training data. Results can be found in Figure~\ref{fig:effi}.
We use 20\%, 40\%, 60\%, and 80\% of the training data from ScanNet and SUN RGB-D dataset. We can observe that our pre-training method gives larger gains when the labeled data is less. And with only ~60\% training data on ScanNet/SUN RGB-D, our model can get similar performance compared with using all training data from scratch. This suggests our pre-training can help the downstream task to obtain better results with fewer data.
\input{figures_tex/efficient}
\input{figures_tex/tsne}

\subsection{Embedding Visualization.} 

We visualize the learned features of our model and baseline approaches in Figure~\ref{fig:tsne}. We compare with FoldingNet~\cite{yang2018foldingnet}, OcCo~\cite{wang2020unsupervised}, and a sanity-check baseline, random initialization. Random initialization use randomly initialized network weight to obtain the embedding, and its performance explains the network prior. The embeddings for different categories in the ModelNet10 dataset are shown using t-SNE dimension reduction. Empirically, we observe that our pre-trained model provides a cleaner separation between different shape categories than FoldingNet~\cite{yang2018foldingnet}, OcCo~\cite{wang2020unsupervised}, and random initialization.

\input{CVPR_2023/sections/08_theory.tex}
