# Supplementary material for: Representation Learning for Point Cloud Understanding
Source: arXiv:2512.06058 source file (2025-12-05)
Supplement: Supplementary file 4 [file supp_cotr_2.tex]

\begin{figure}[h]
    \begin{center}
    \includegraphics[width=1\linewidth]{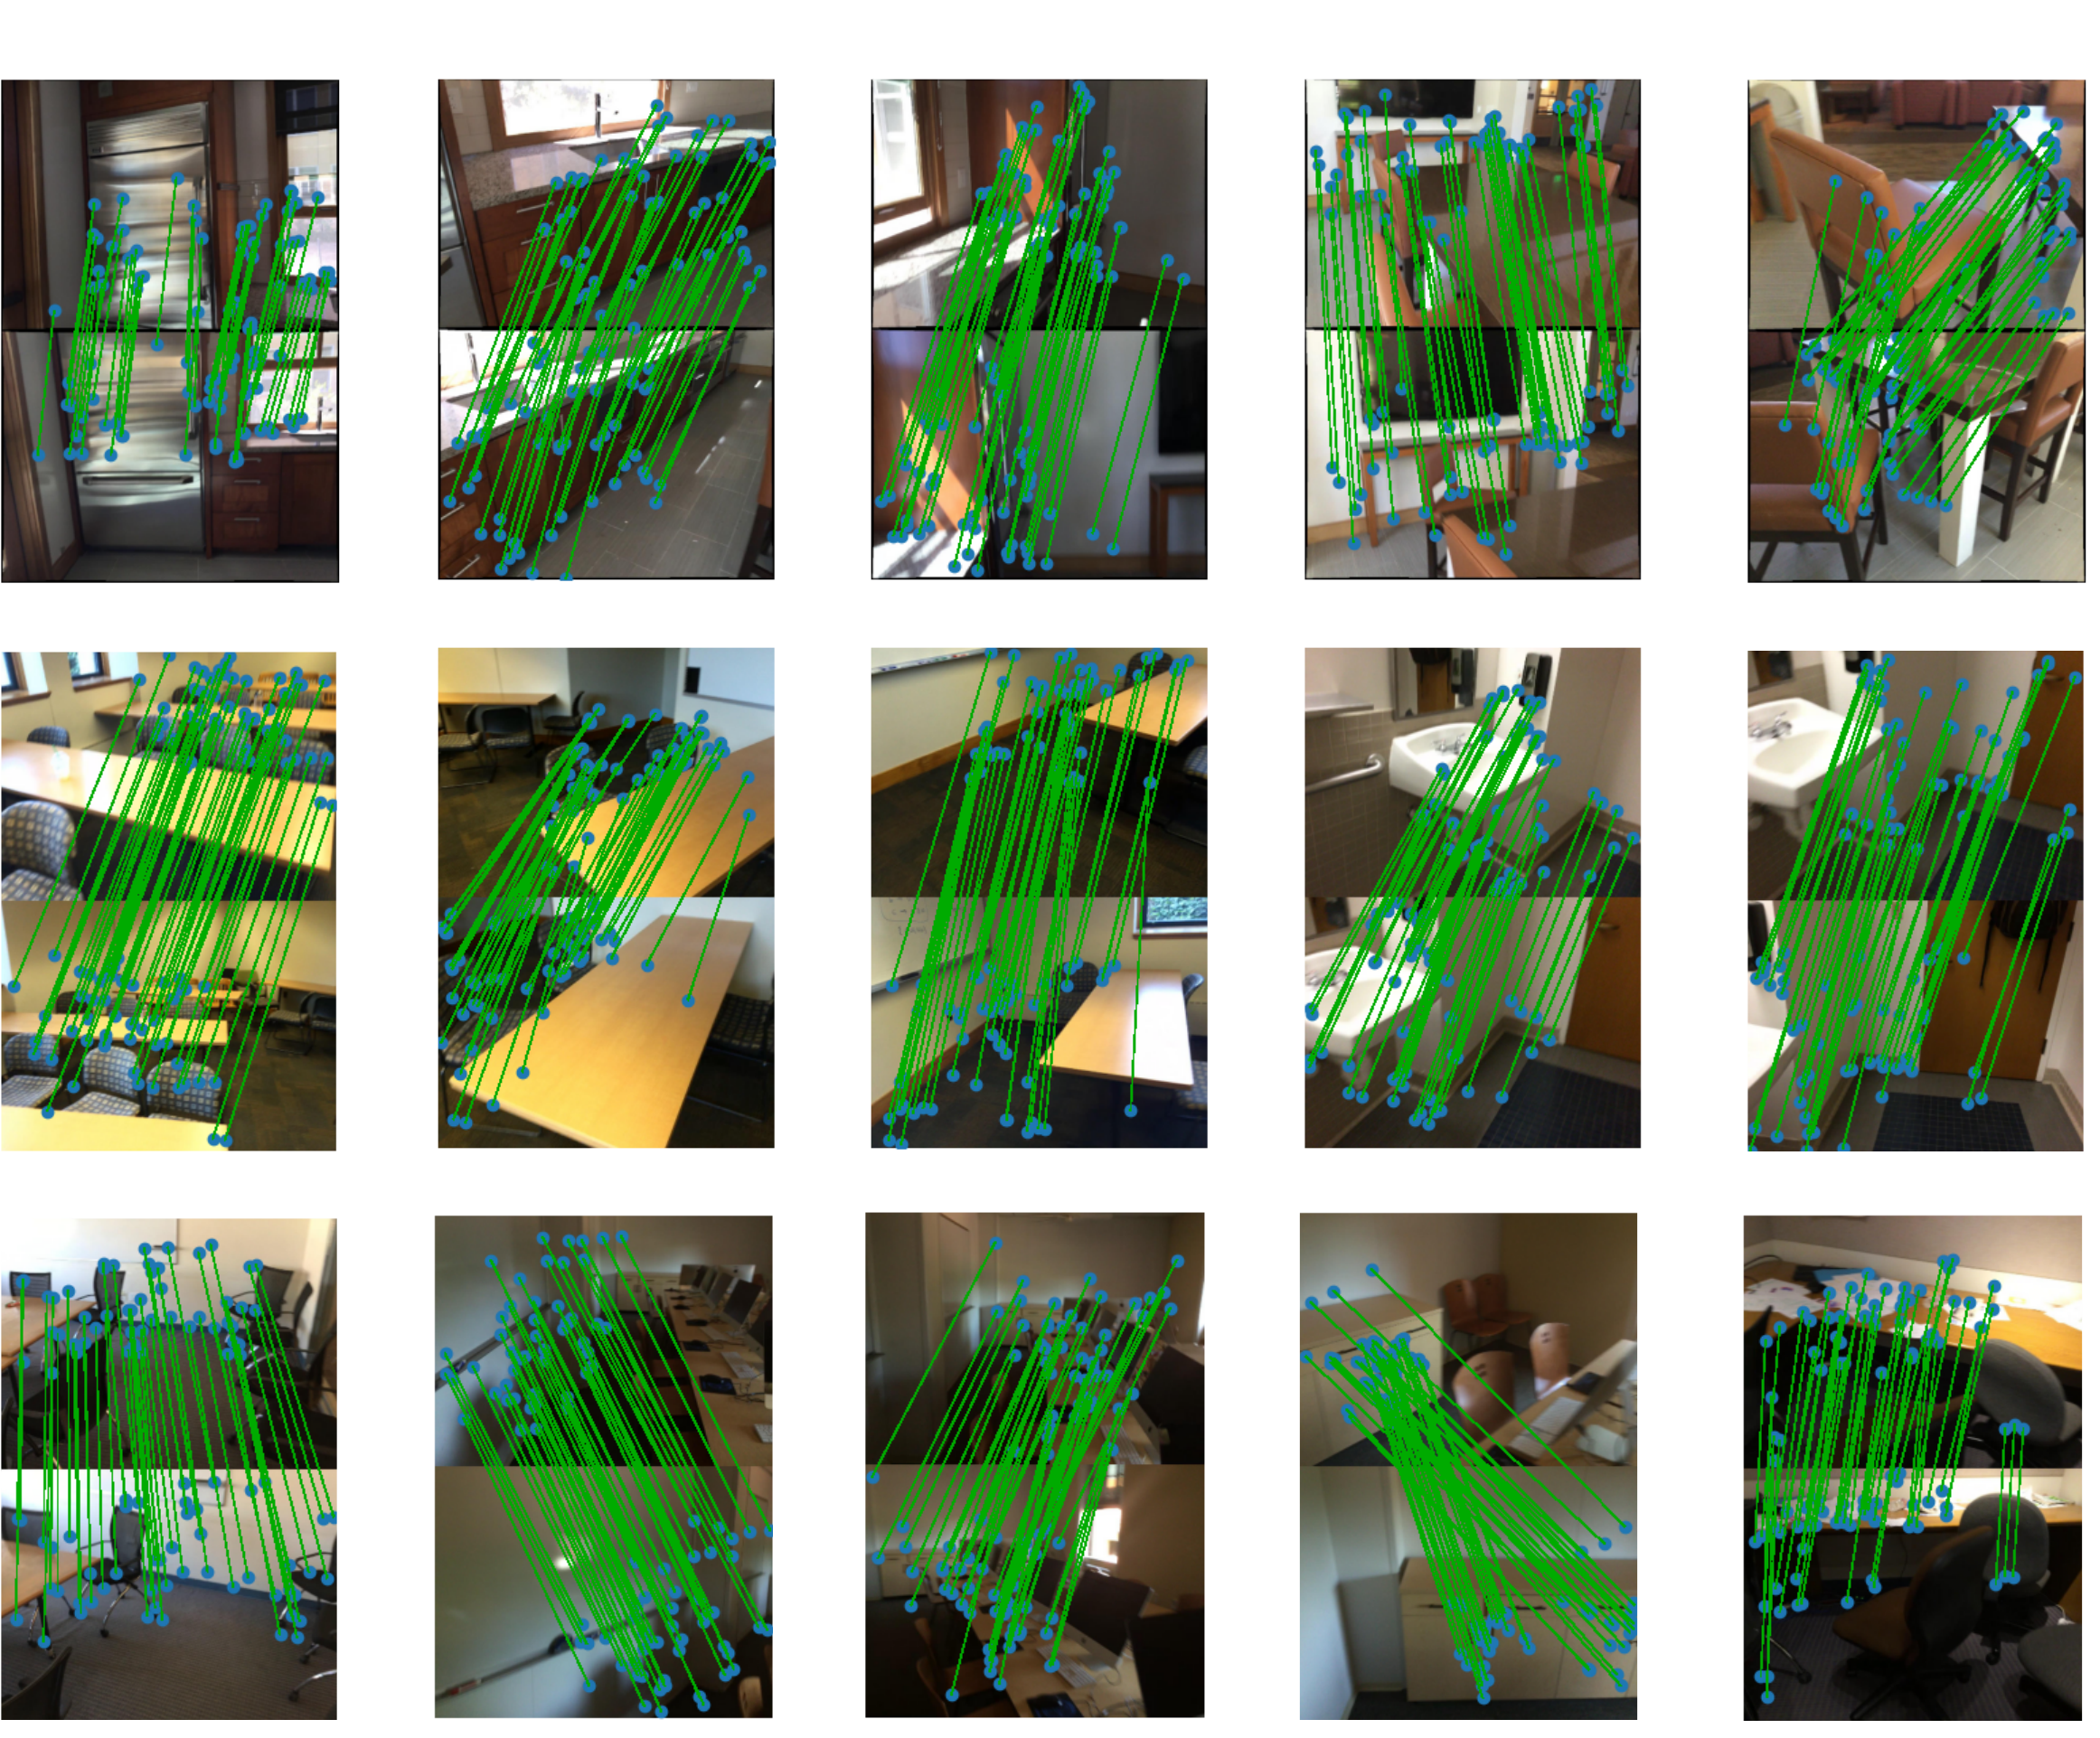}
    \end{center}
    \caption{\textbf{Qualitative results of multi-view consistency module prediction.} Each element consists of two different view images. The query points and prediction points are visualized using the blue dot, and they are connected by the green line.}
    \label{Fig:supp_cotr}
\end{figure}
