# Supplementary material for: Representation Learning for Point Cloud Understanding
Source: arXiv:2512.06058 source file (2025-12-05)
Supplement: Supplementary file 5 [file supp_eff.tex]

\begin{figure}[h]
    \begin{center}
    \includegraphics[width=1\linewidth]{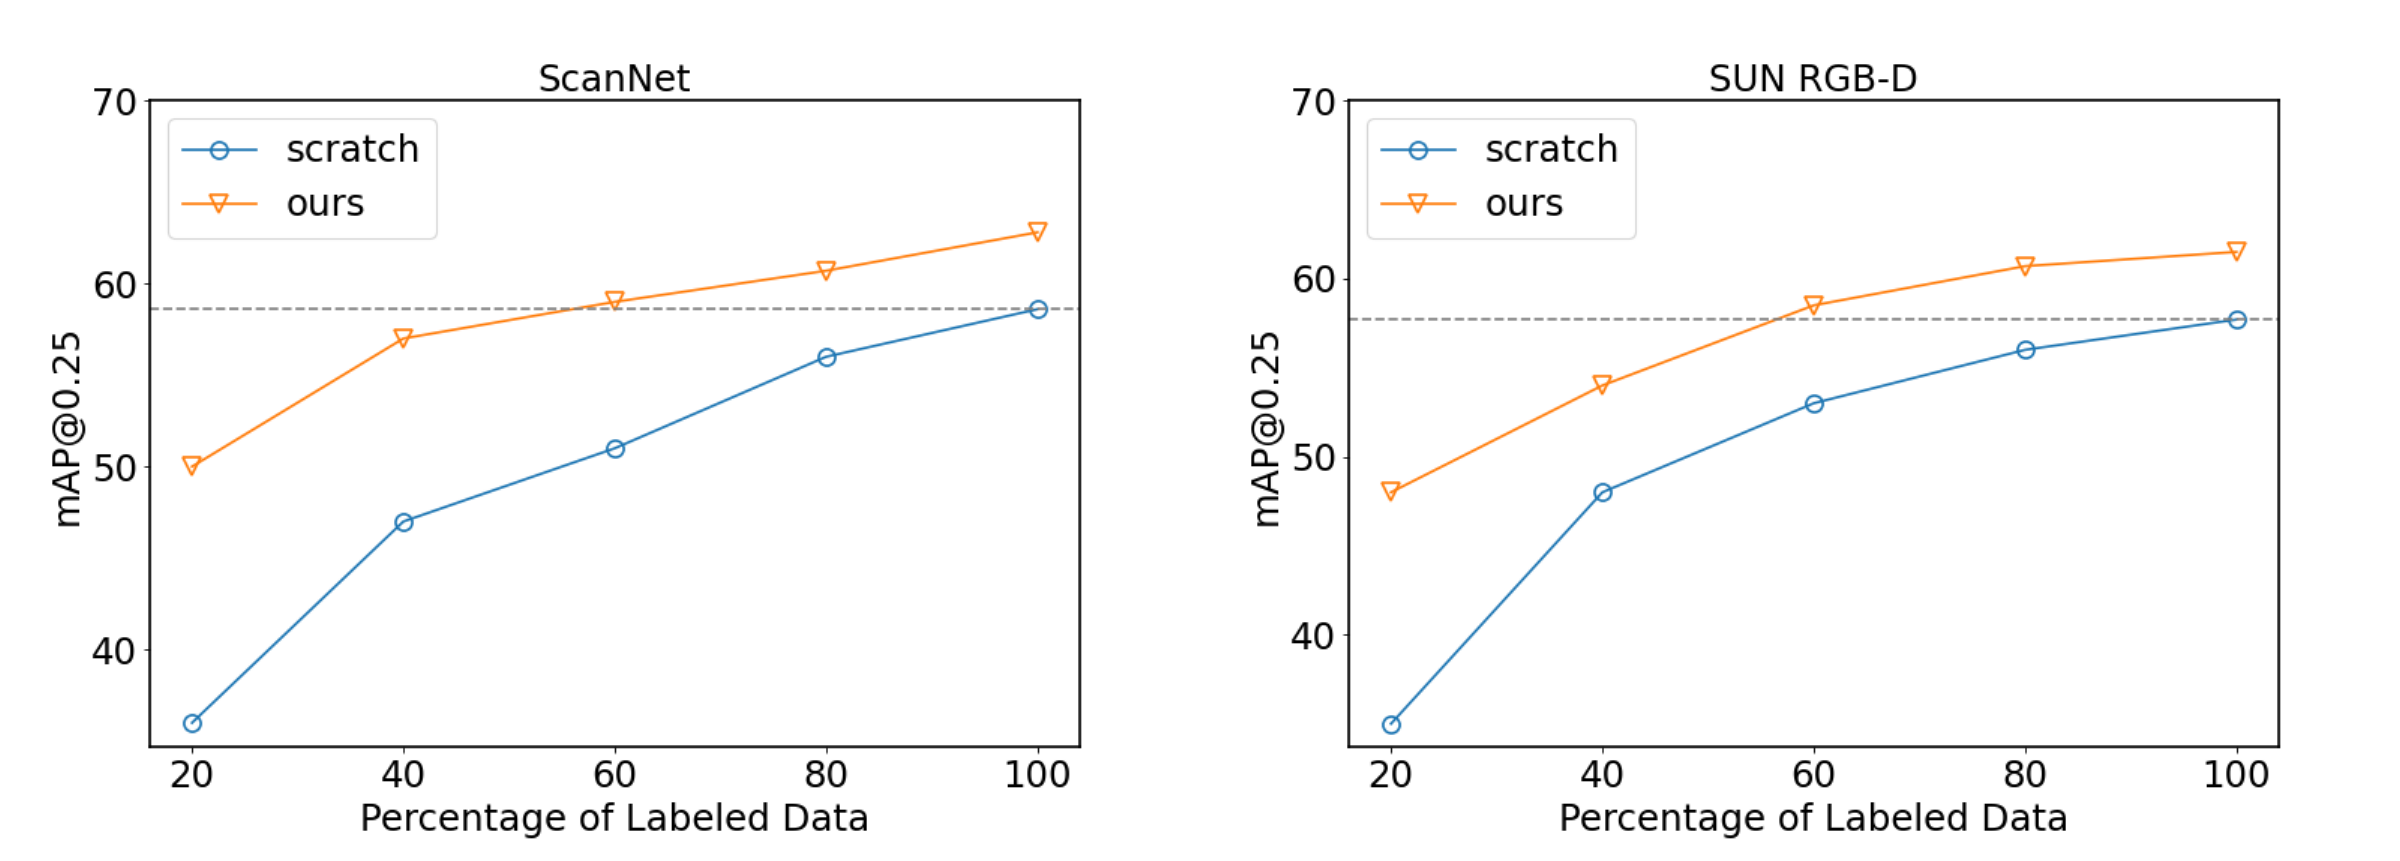}
    \end{center}
    \caption{\textbf{Illustration of Label efficiency training.} Our model is pre-trained on ScanNet and subsequently fine-tuned separately on both ScanNet and SUN RGBD. We take VoteNet as network architecture. During this fine-tuning process, we employ varying percentages of labeled training data. Demonstrating its efficacy, our pre-training model not only surpasses the performance of models trained from scratch but also achieves comparable results utilizing only 60\% of the labeled data.}
    \label{fig:eff}
\end{figure}
