# Supplementary material for: Representation Learning for Point Cloud Understanding
Source: arXiv:2512.06058 source file (2025-12-05)
Supplement: Supplementary file 6 [file supp_qual.tex]

\begin{figure}[h]
    \begin{center}
    \includegraphics[width=\linewidth]{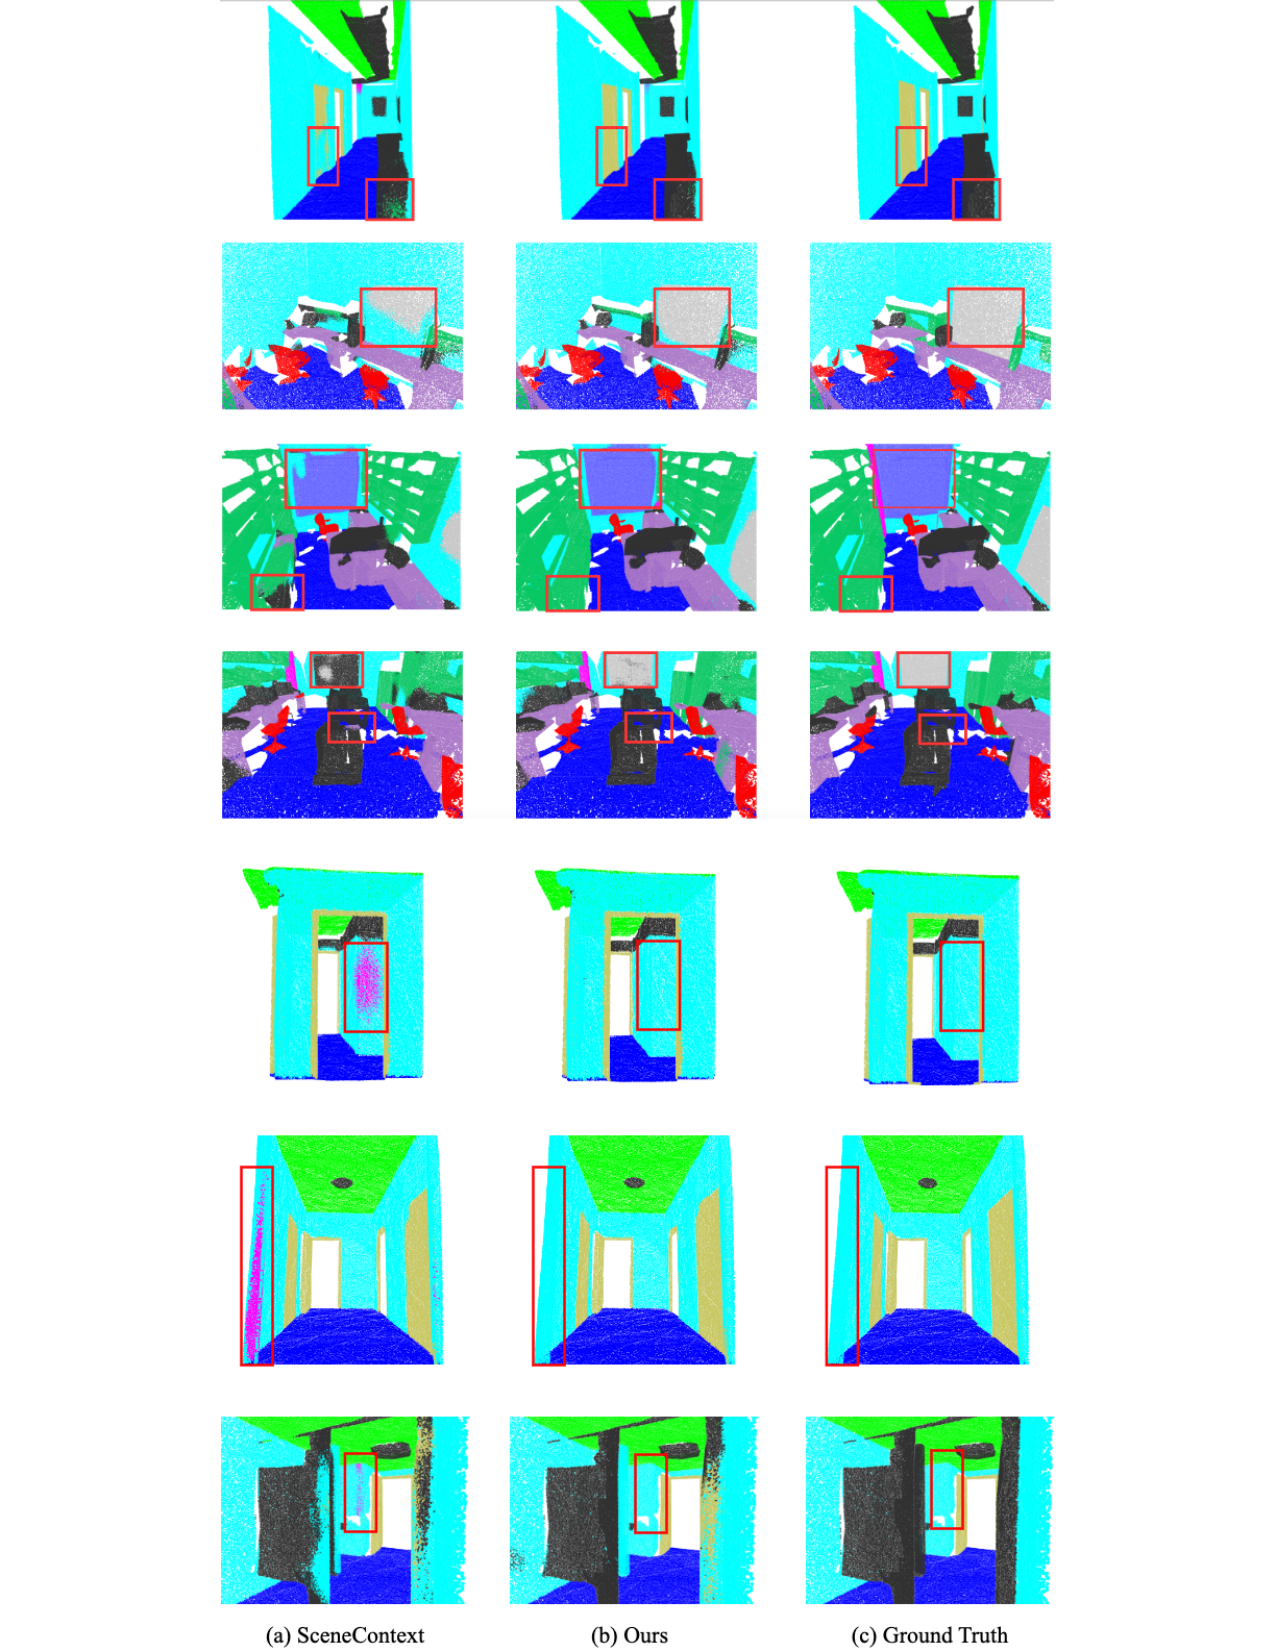}
    \end{center}
    \caption{\textbf{Qualitative results on S3DIS semantic segmentation task.} We compare our method with the second-best approach, SceneContext~\citep{hou2021exploring}.}
    \label{Fig:srnet}
\end{figure}
