# Supplementary material for: Representation Learning for Point Cloud Understanding
Source: arXiv:2512.06058 source file (2025-12-05)
Supplement: Supplementary file 8 [file supp_radar_chart.tex]

\begin{figure}[h]
    \centering   
    \includegraphics[width=0.7\linewidth]{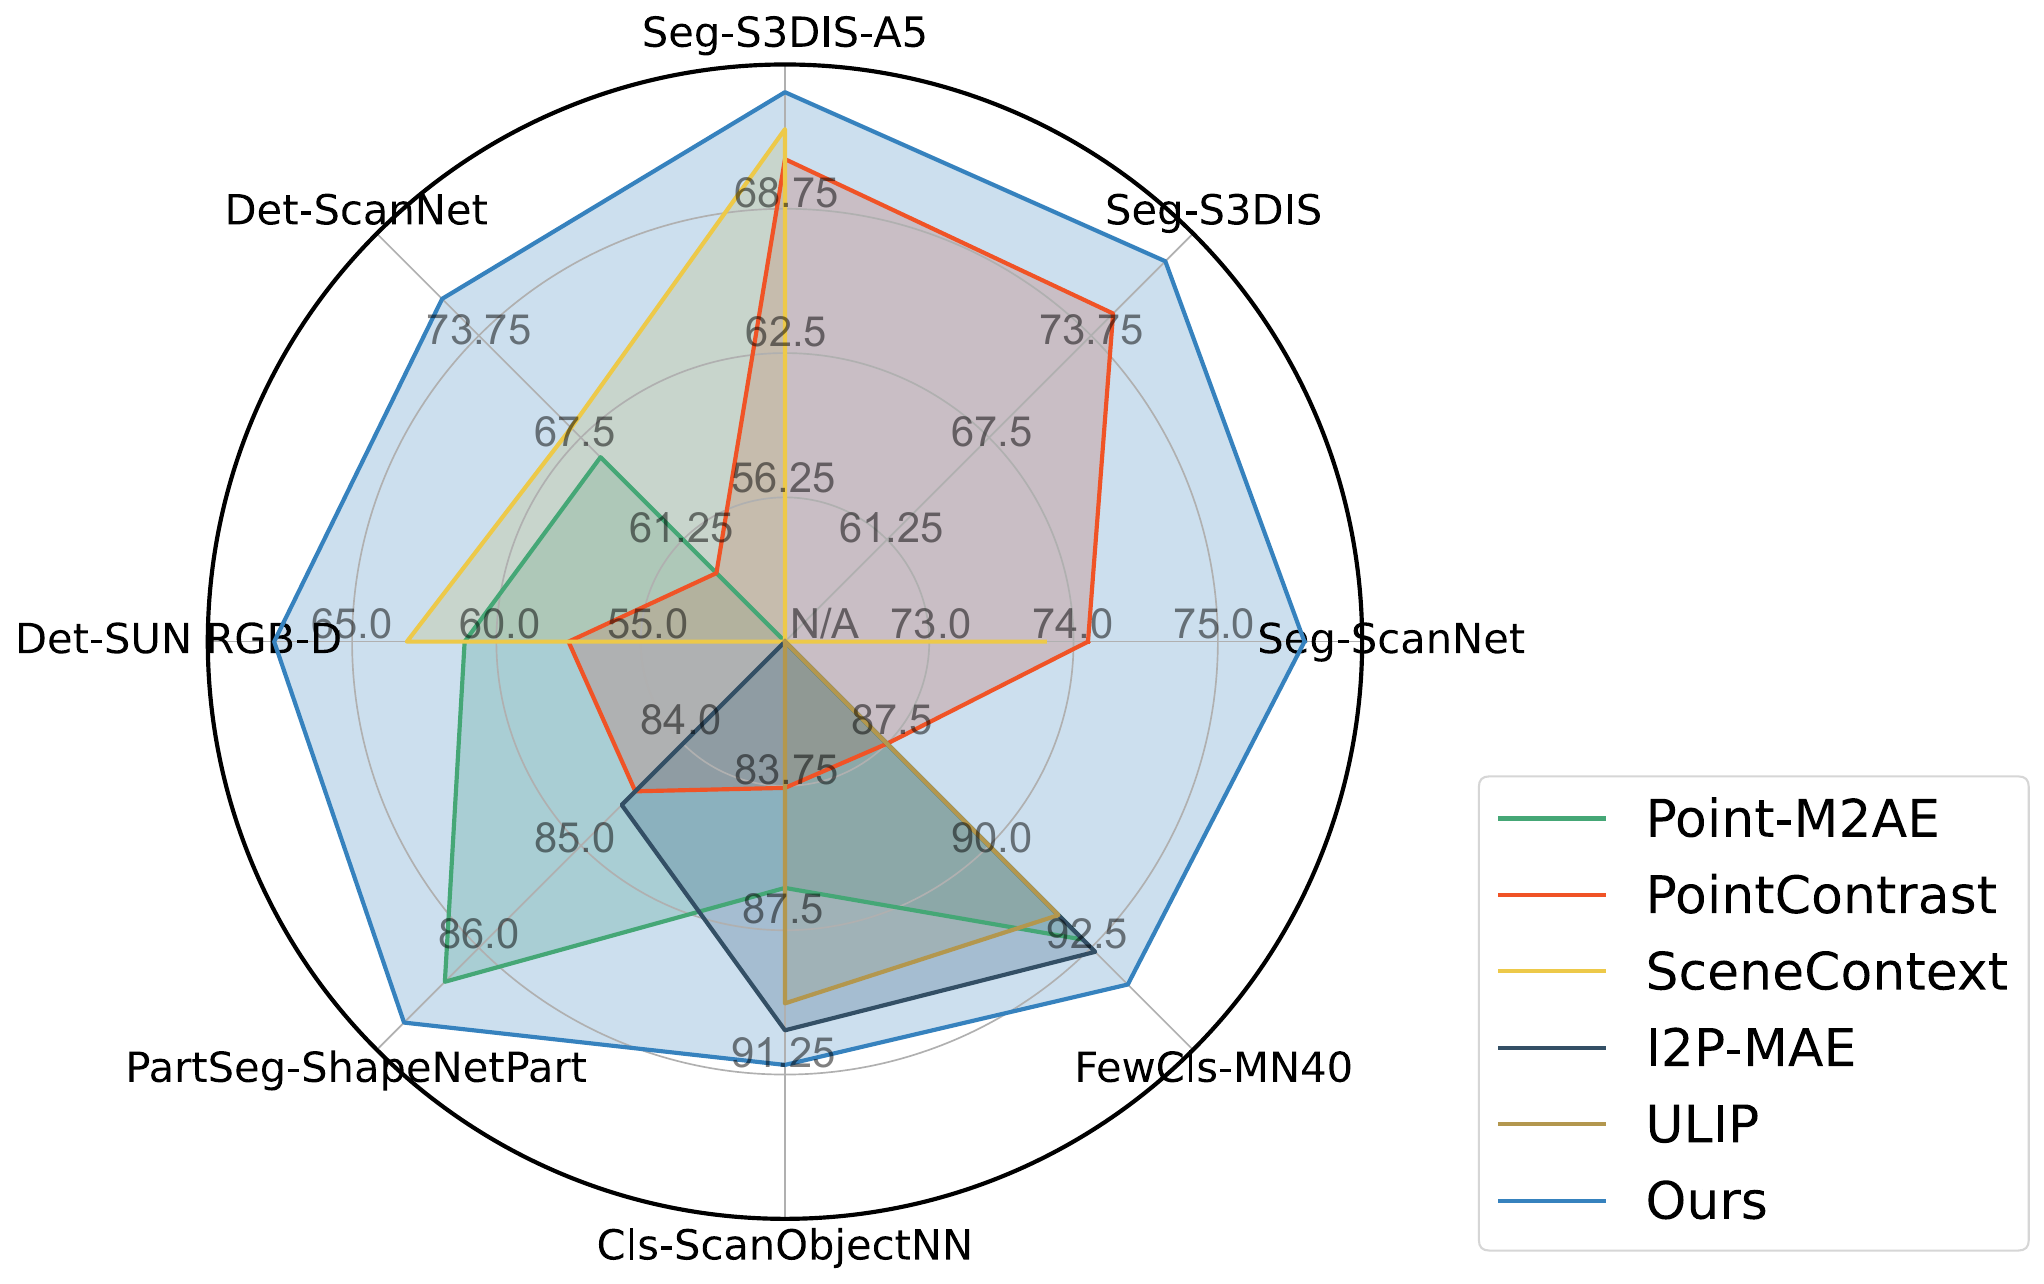}
    %\caption{Our model (blue) achieves state-of-the-art performance across a broad range of tasks at both the scene and shape levels. The distance to the origin indicates the task result.}
    \label{fig:radar}
\end{figure}
