# Supplementary material for: Representation Learning for Point Cloud Understanding
Source: arXiv:2512.06058 source file (2025-12-05)
Supplement: Supplementary file 9 [file supp_srnet.tex]

\begin{figure}[h]
    \begin{center}
    \includegraphics[width=1\linewidth]{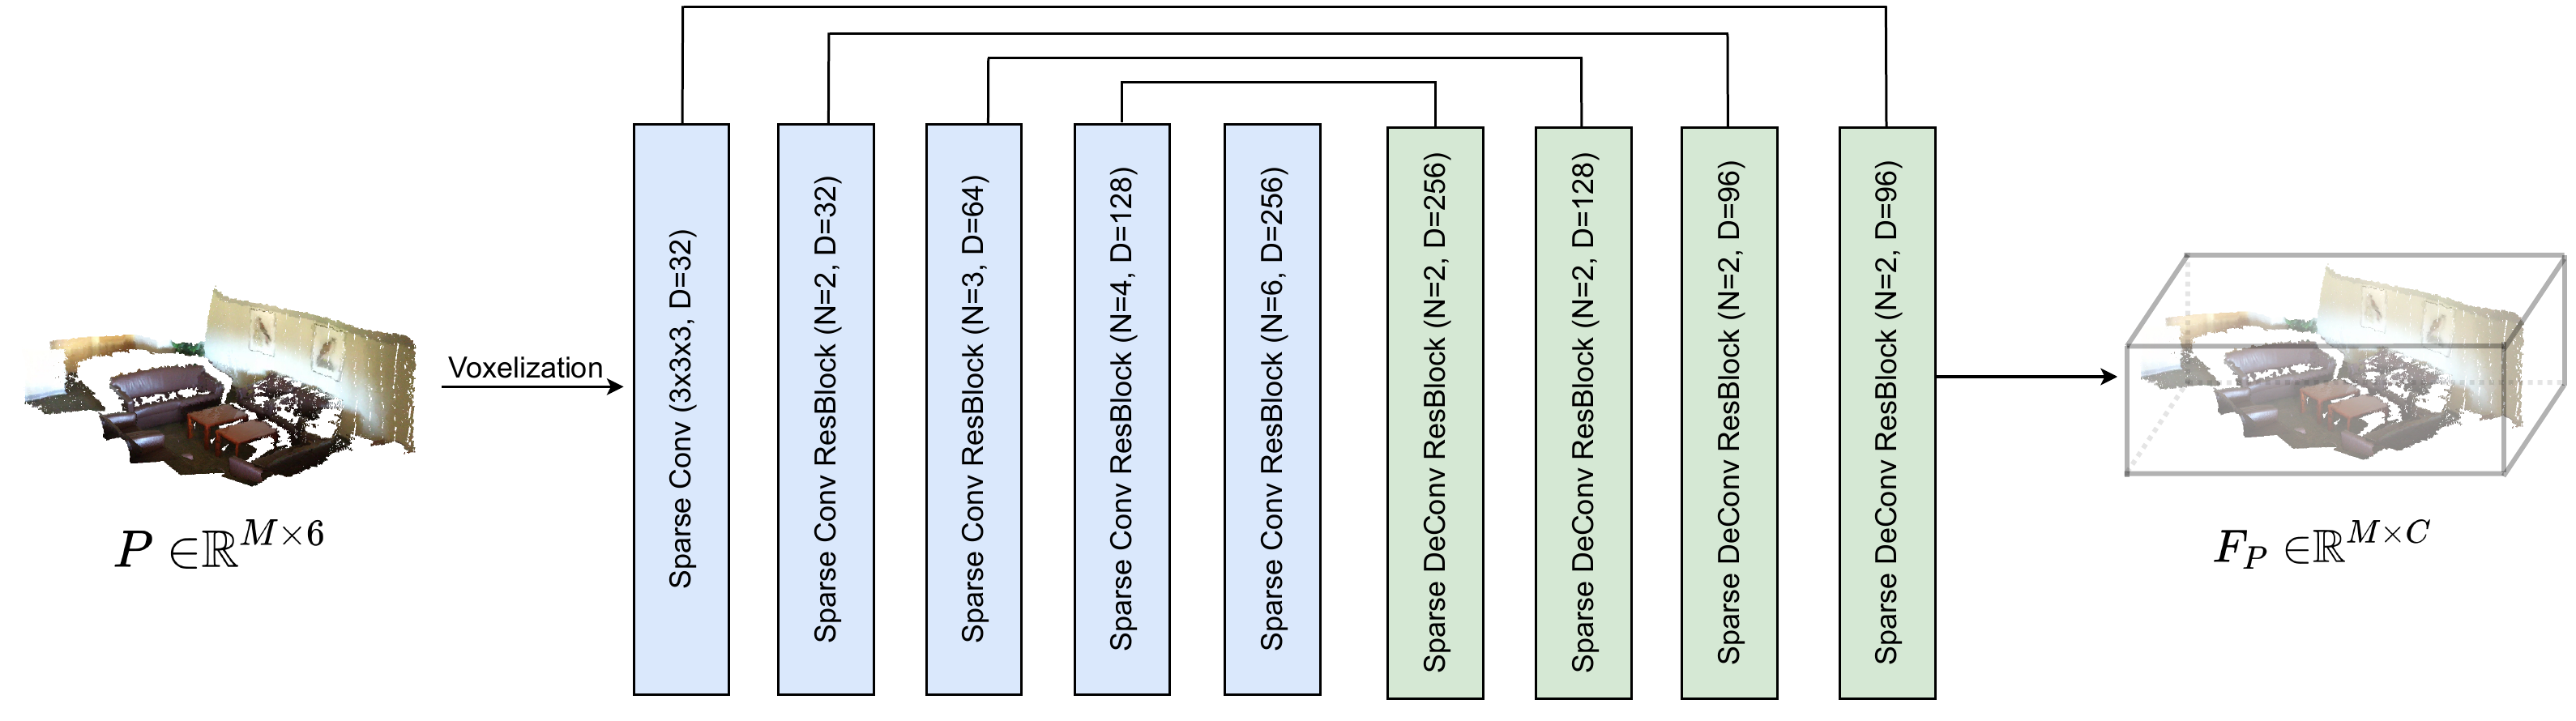}
    \end{center}
    \caption{\textbf{Feature encoding network details.}}
    \label{Fig:srnet}
\end{figure}
