# Supplementary material for: Representation Learning for Point Cloud Understanding
Source: arXiv:2512.06058 source file (2025-12-05)
Supplement: Supplementary file 10 [file supp_fewshot.tex]

\begin{table*}[t]
\centering
\setlength\tabcolsep{8pt}% 调整列间距
\scriptsize

\begin{tabular}{lcccc}
\toprule
\multirow{2}{*}{\textbf{Method}} & \multicolumn{2}{c}{\textbf{5-way}} & \multicolumn{2}{c}{\textbf{10-way}} \\
\cmidrule(lr){2-3}   \cmidrule(lr){4-5}
 & 10-shot & 20-shot & 10-shot & 20-shot \\
\hline
DGCNN$^{\dagger}$ & $31.6 \pm 2.8$ & $40.8 \pm 4.6$ & $19.9 \pm 2.1$ & $16.9 \pm 1.5$ \\
OcCo & $90.6 \pm 2.8$ & $92.5 \pm 1.9$ & $82.9 \pm 1.3$ & $86.5 \pm 2.2$ \\
CrossPoint & $92.5 \pm 3.0$ & $94.9 \pm 2.1$ & $83.6 \pm 5.3$ & $87.9 \pm 4.2$ \\
\hline
Transformer$^{\dagger}$ & $87.8 \pm 5.2$ & $93.3 \pm 4.3$ & $84.6 \pm 5.5$ & $89.4 \pm 6.3$ \\
OcCo & $94.0 \pm 3.6$ & $95.9 \pm 2.3$ & $89.4 \pm 5.1$ & $92.4 \pm 4.6$ \\
PointBERT & $94.6 \pm 3.1$ & $96.3 \pm 2.7$ & $91.0 \pm 5.4$ & $92.7 \pm 5.1$ \\
MaskDiscr & $95.0 \pm 3.7$ & $97.2 \pm 1.7$ & $91.4 \pm 4.0$ & $93.4 \pm 3.5$ \\
PointMAE & $96.3 \pm 2.5$ & $97.8 \pm 1.8$ & $92.6 \pm 4.1$ & $95.0 \pm 3.0$ \\
\rowcolor{gray!20} MVNet & $\pmb{97.2} \pm \pmb{1.8}$ & $\pmb{98.3} \pm \pmb{1.8}$ &  $\pmb{93.4} \pm \pmb{3.4}$ & $\pmb{95.8} \pm \pmb{3.2}$ \\
\bottomrule
\end{tabular}
\caption{\small{\textbf{Few-shot classification on ModelNet40.} We report the average accuracy (\%) and standard deviation (\%) of 10 independent experiments. $^{\dagger}$ represents the \textit{from scratch} results and all other methods represent the \textit{fine-tuning} results using pretrained weights.}}
\label{tab:mn_fewshot}

\end{table*}
