# Supplementary material for: Representation Learning for Point Cloud Understanding
Source: arXiv:2512.06058 source file (2025-12-05)
Supplement: Supplementary file 12 [file supp_shape_task.tex]

\begin{table*}[t]
    \centering
    \resizebox{1.\linewidth}{!}{  
    \footnotesize
    \begin{tabular}{llccccc}
        \toprule
        \multirow{2}{*}{Method} & \multirow{2}{*}{Backbone} & \multicolumn{3}{c}{ScanObjectNN} & \multicolumn{2}{c}{ShapeNetPart} \\
        \cmidrule(lr){3-5} \cmidrule(lr){6-7} & & OBJ-BG & OBJ-ONLY & PB-T50-RS & ins. mIoU & cls. mIoU \\
        \midrule
        Jigsaw~\citep{sauder2019self} & DGCNN & 86.8 & 86.2 & 83.5 & 85.3 & - \\
        OcCo~\citep{wang2020unsupervised} & DGCNN & 88.2& 87.5 & 85.0 &  - \\
        CrossPoint~\citep{afham2022crosspoint} & DGCNN & - & - & 85.5 & 83.7\\
        ULIP~\citep{xue2023ulip} & Transformer & 91.3 & 89.4 & 86.4 & - & -\\
        ULIP~\citep{xue2023ulip} & PointMLP & 93.2 & 90.4 & 89.4 & - & -\\
        Point-M2AE~\citep{zhang2022point} & M2AE & 91.2 & 88.8 & 86.4 & 86.5 & 84.9\\
        I2P-MAE~\cite{zhang2023learning} & M2AE & 94.2 & 91.6 & 90.1 & \textbf{86.8} & \textbf{85.2}\\
        \rowcolor{gray!20}MVNet-L & Transformer & \textbf{95.2} & \textbf{94.2}  & \textbf{91.0} & \textbf{86.8} & \textbf{85.2} \\
        \bottomrule
    \end{tabular}
    }
    % \vspace{5pt}
    \vspace{-2mm}
    \caption{\small{\textbf{Performance comparison with pre-training approaches using different network backbones on shape-level downstream tasks.} }}
    \label{tab:supp-shape-result}
    %\vspace{-3pt}
\end{table*}
