# Supplementary material for: Representation Learning for Point Cloud Understanding
Source: arXiv:2512.06058 source file (2025-12-05)
Supplement: Supplementary file 15 [file supp-fig-sv.tex]

\begin{figure*}[t]
\centering
\footnotesize

\def\imw{0.17\textwidth}
\def\imww{0.15\textwidth}
\newcommand{\T}[1]{\raisebox{-0.5\height}{#1}}
\setlength{\tabcolsep}{1pt}
\begin{tabular}{cccccc}
\T{\includegraphics[width=\imw]{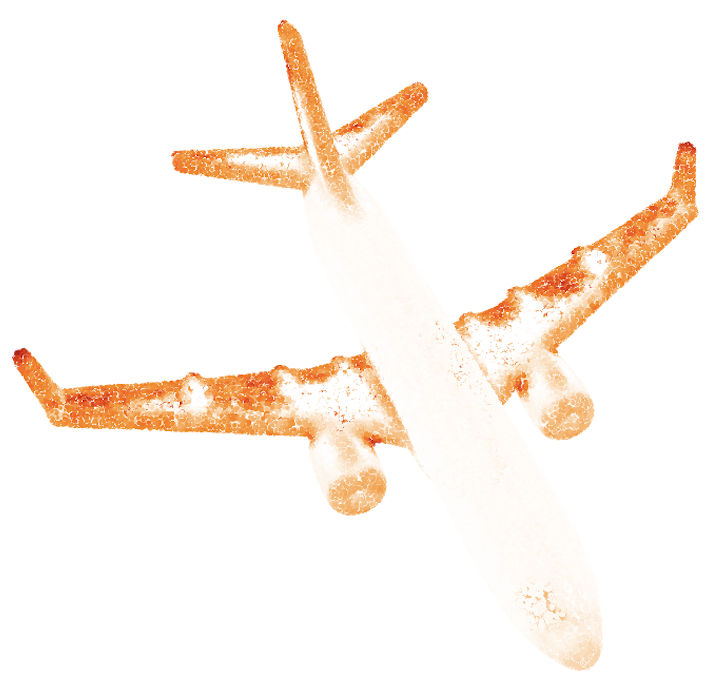}} &
\T{\includegraphics[width=\imw]{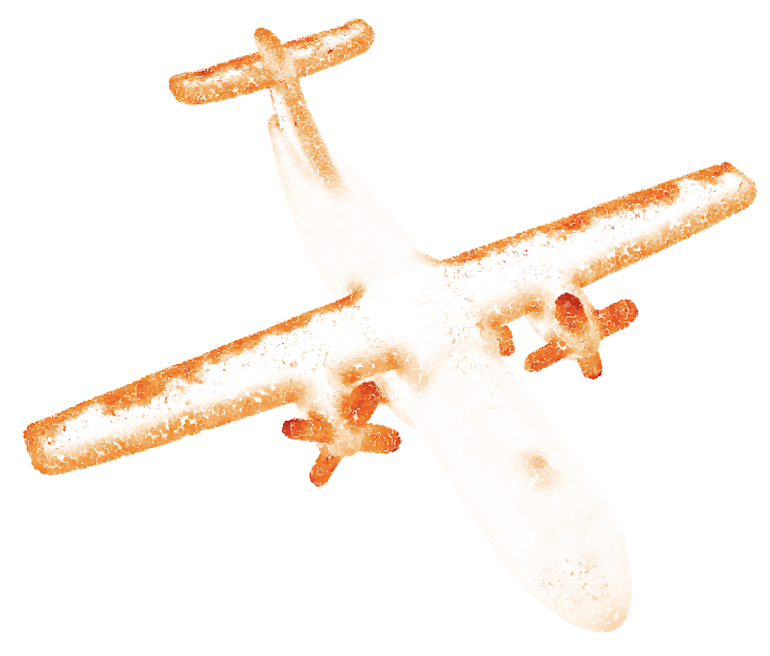}} &
\T{\includegraphics[width=\imw]{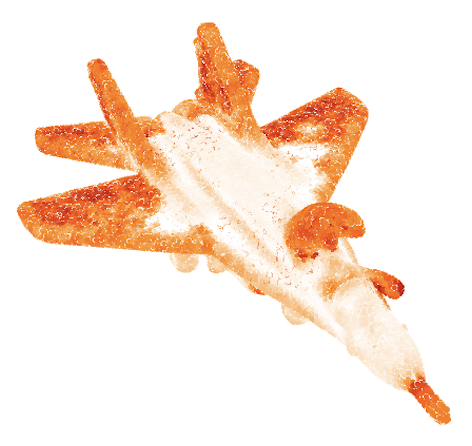}} &
\T{\includegraphics[width=\imw]{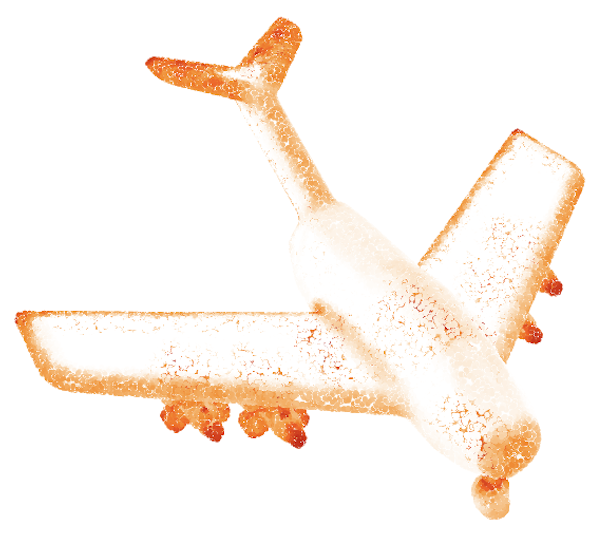}} &
\T{\includegraphics[width=\imw] {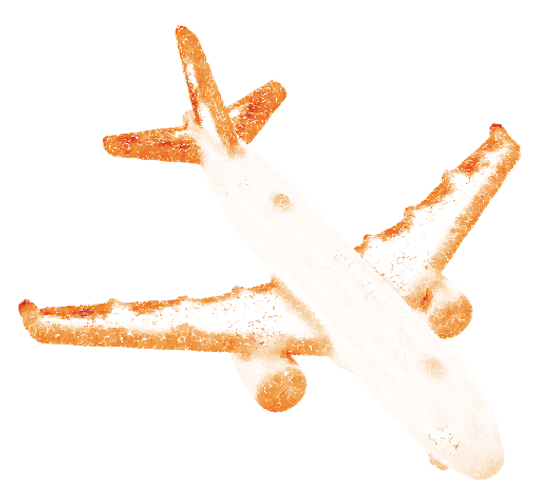}} &
%\T{\includegraphics[width=\imw] {Images/sv_vis/airplane5.png}} &
\T{\includegraphics[width=\imw] {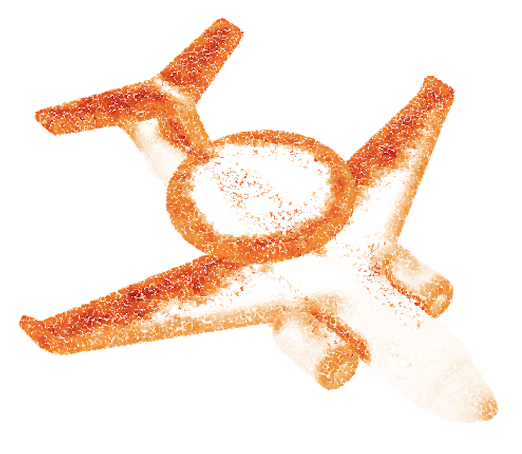}} 
\\ 
\T{\includegraphics[width=\imw]{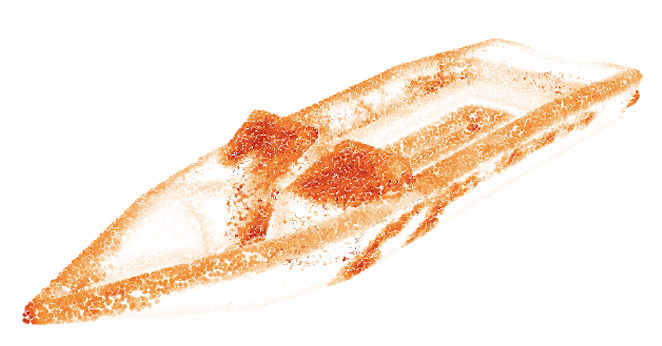}} &
\T{\includegraphics[width=\imw]{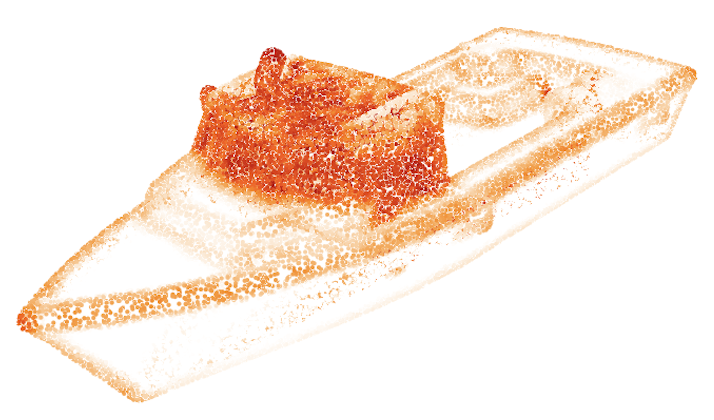}} &
\T{\includegraphics[width=\imw]{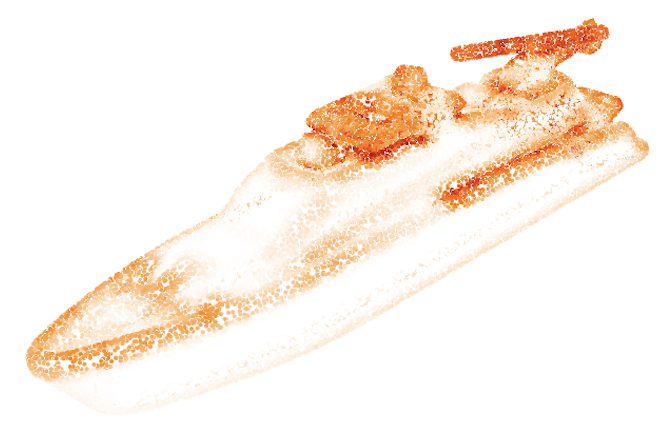}} &
\T{\includegraphics[width=\imw]{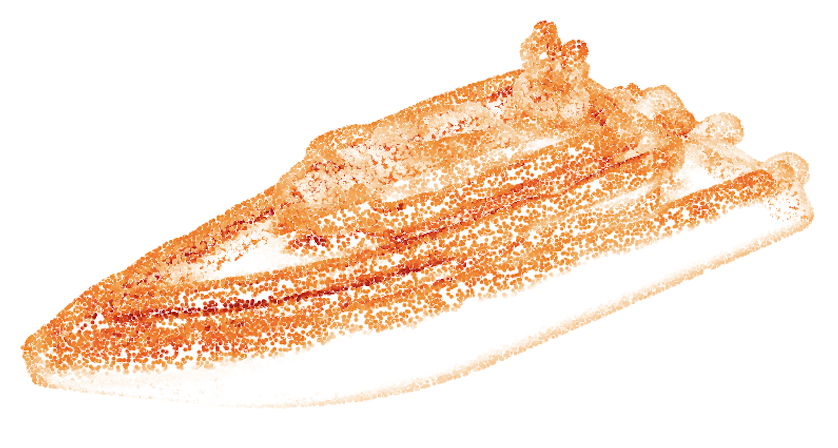}} &
\T{\includegraphics[width=\imw] {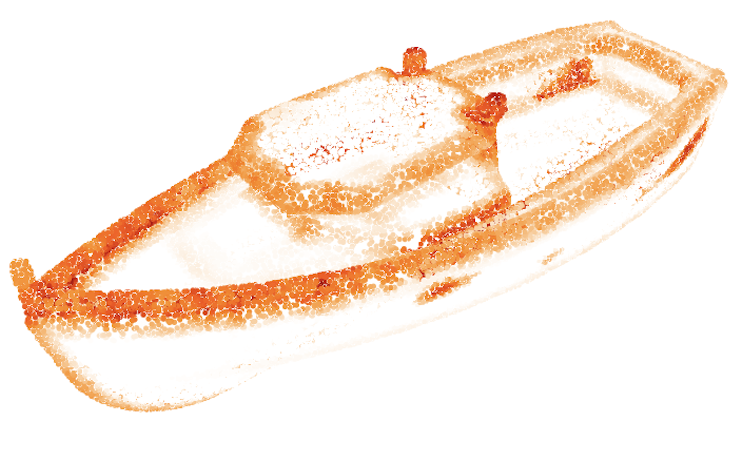}} &
%\T{\includegraphics[width=\imw] {Images/sv_vis/airplane5.png}} &
\T{\includegraphics[width=\imw] {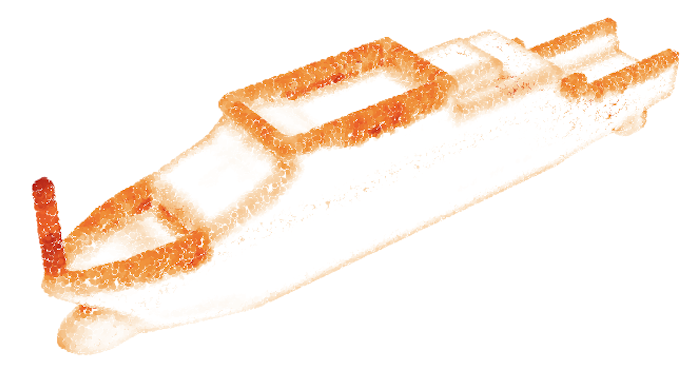}} 
\\ 
\T{\includegraphics[width=\imw]{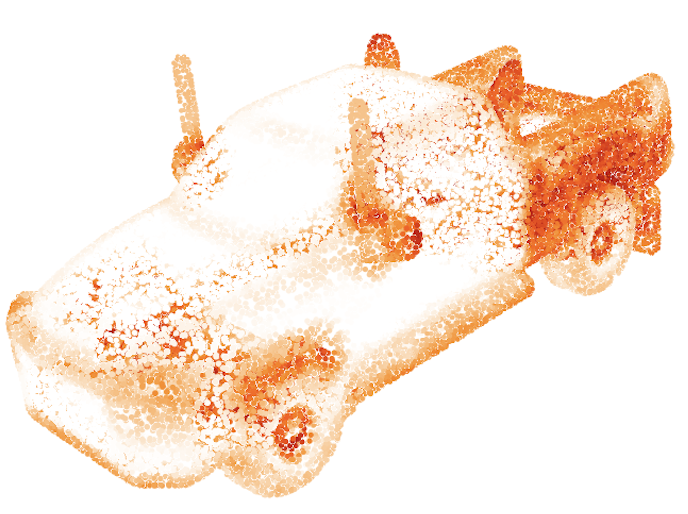}} &
\T{\includegraphics[width=\imw]{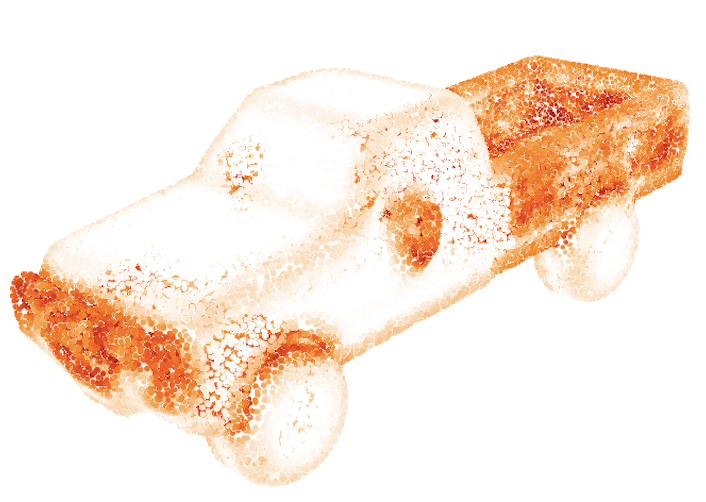}} &
\T{\includegraphics[width=\imw]{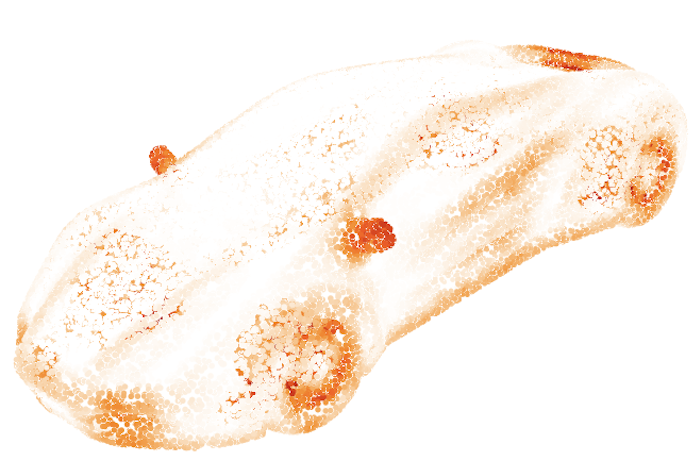}} &
\T{\includegraphics[width=\imw]{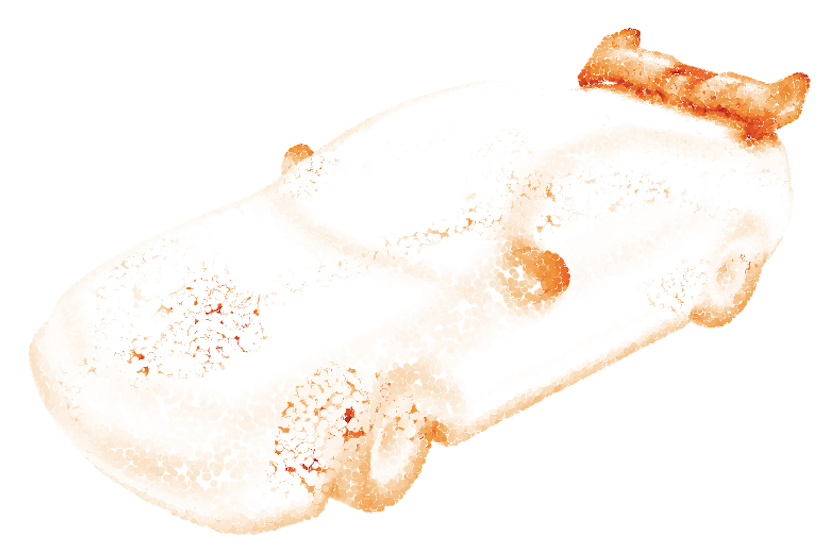}} &
\T{\includegraphics[width=\imw] {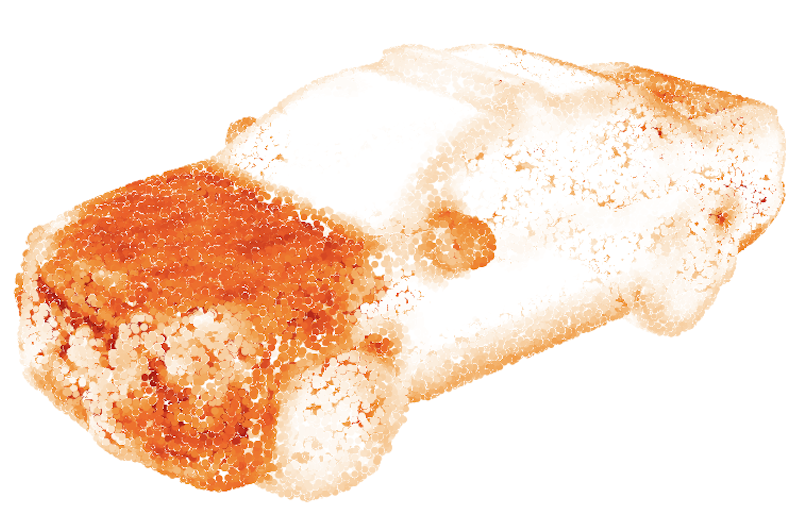}} &
%\T{\includegraphics[width=\imw] {Images/sv_vis/airplane5.png}} &
\T{\includegraphics[width=\imw] {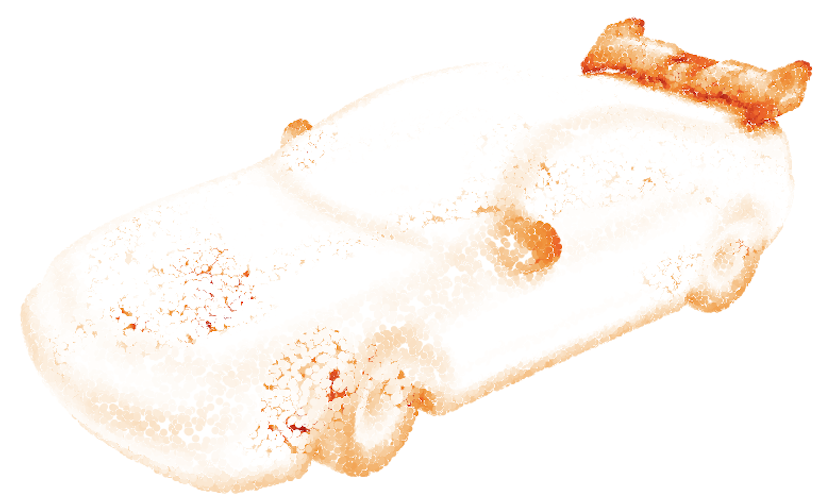}} 
\\ 
\T{\includegraphics[width=\imw]{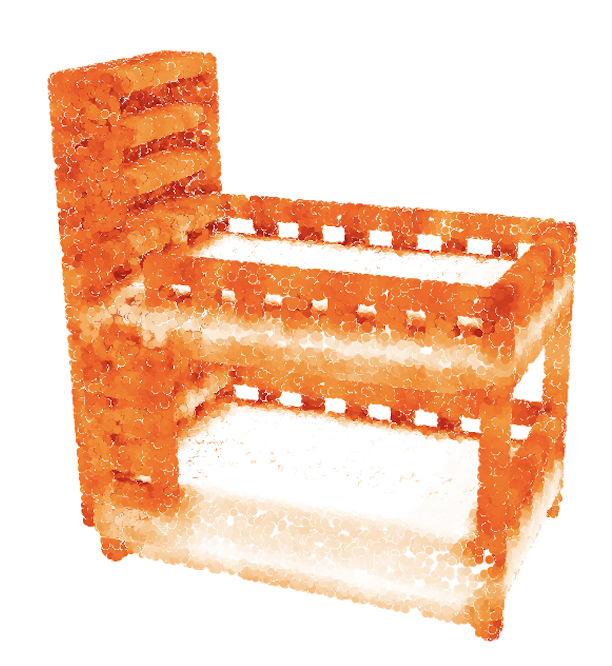}} &
\T{\includegraphics[width=\imw]{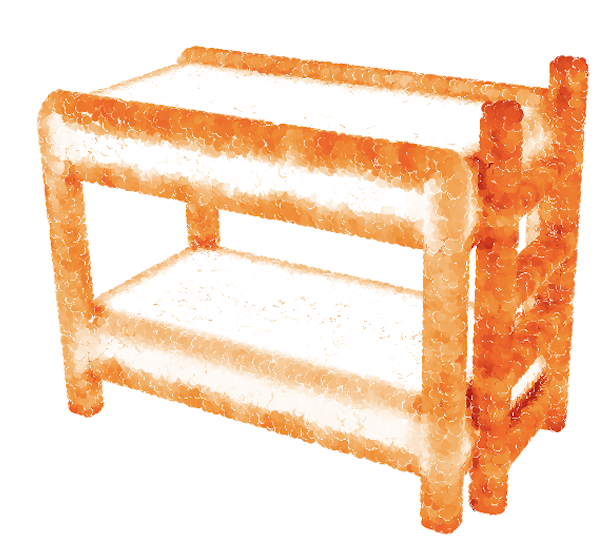}} &
\T{\includegraphics[width=\imw]{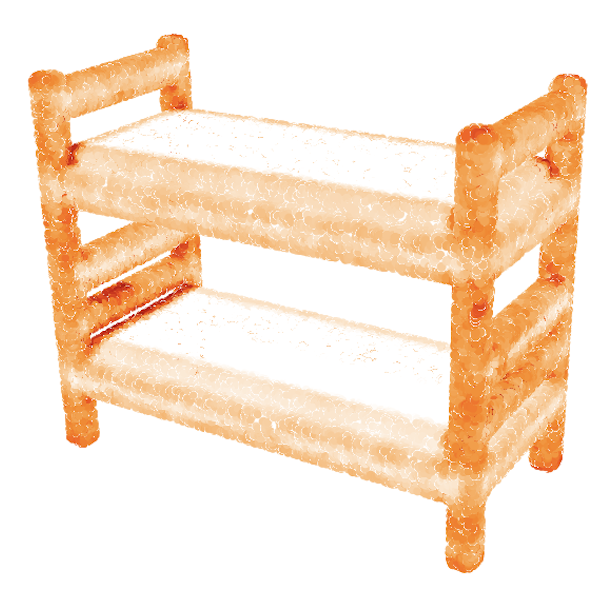}} &
\T{\includegraphics[width=\imw]{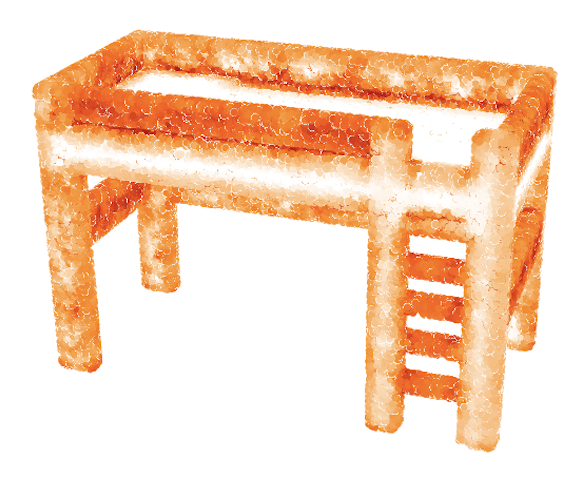}} &
\T{\includegraphics[width=\imw] {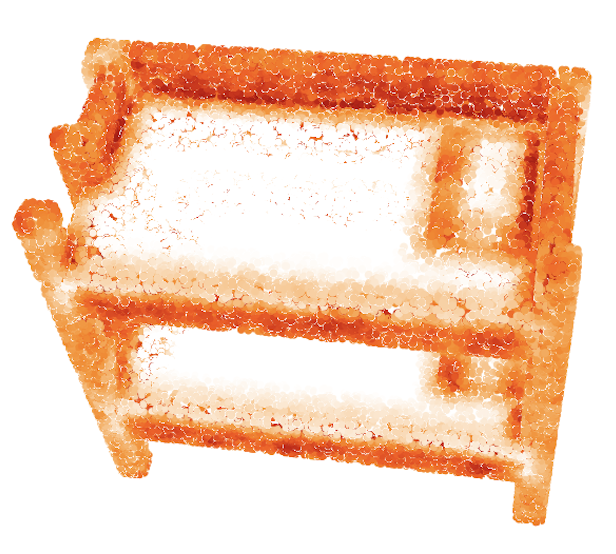}} &
%\T{\includegraphics[width=\imw] {Images/sv_vis/airplane5.png}} &
\T{\includegraphics[width=\imw] {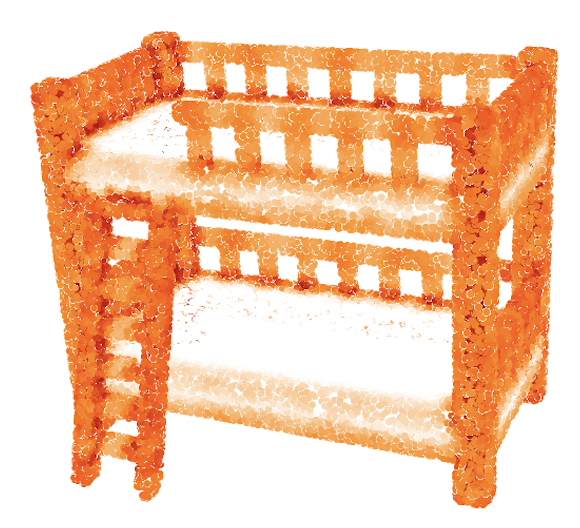}} 
\\ 
\T{\includegraphics[width=\imw]{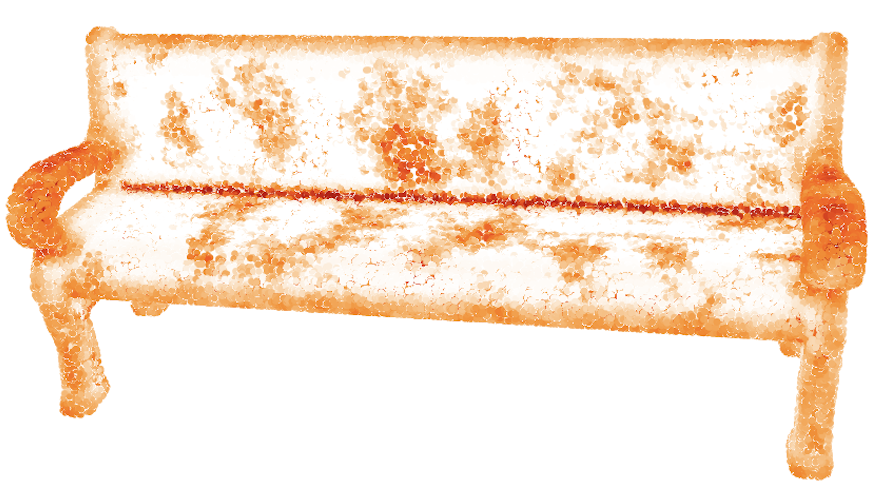}} &
\T{\includegraphics[width=\imw]{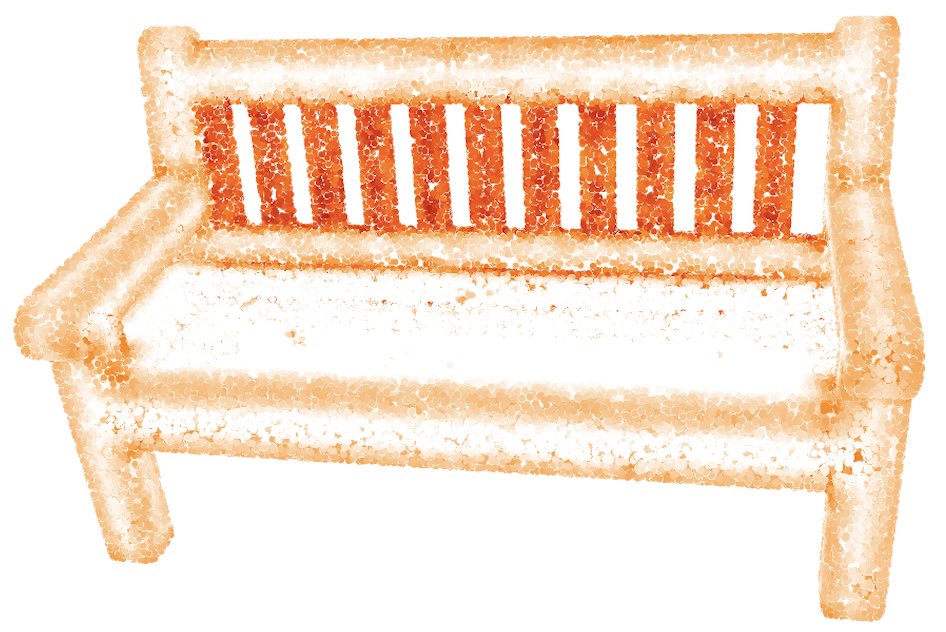}} &
\T{\includegraphics[width=\imw]{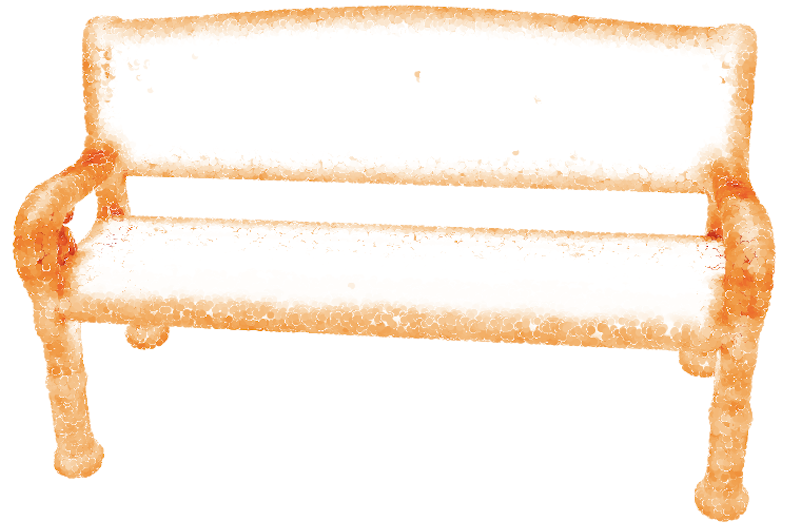}} &
\T{\includegraphics[width=\imw]{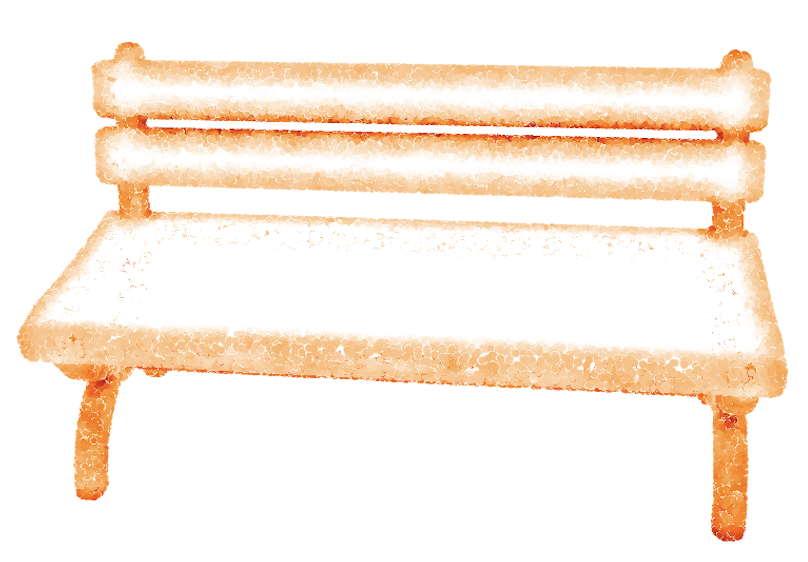}} &
\T{\includegraphics[width=\imw] {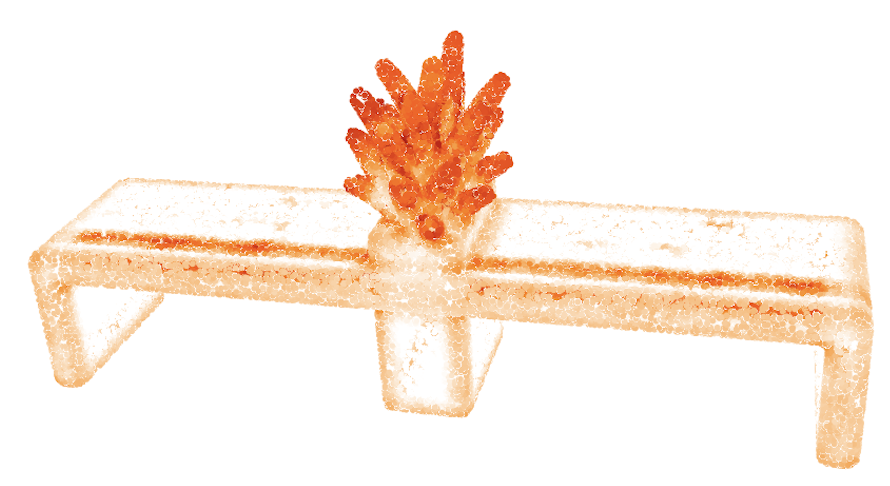}} &
%\T{\includegraphics[width=\imw] {Images/sv_vis/airplane5.png}} &
\T{\includegraphics[width=\imw] {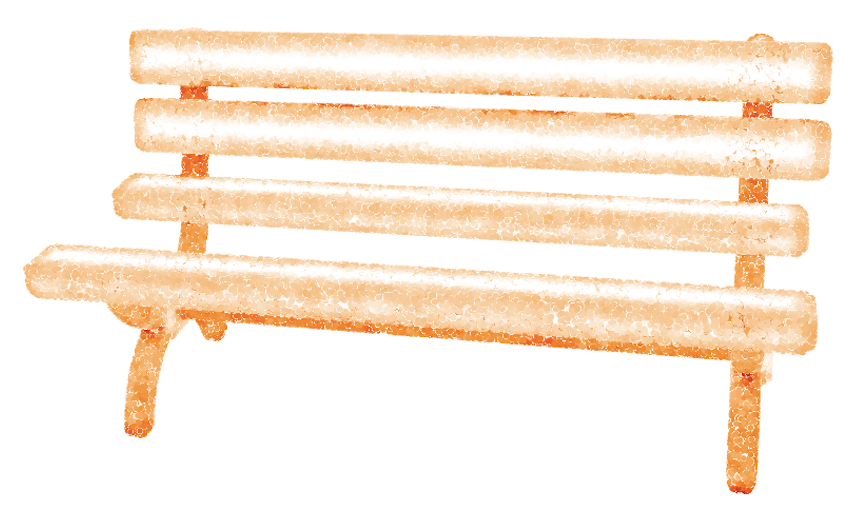}} 
\\
\T{\includegraphics[width=\imww]{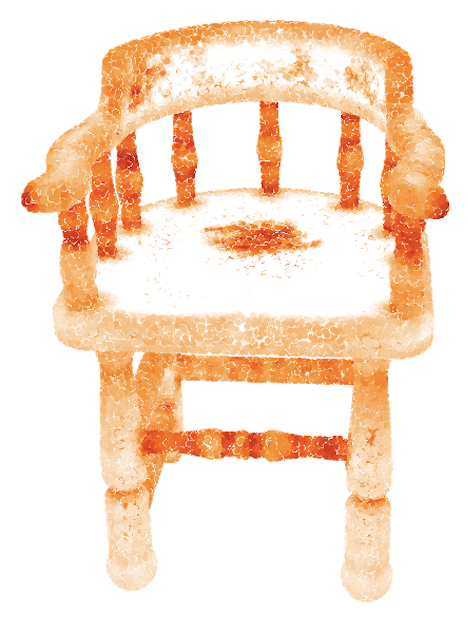}} &
\T{\includegraphics[width=\imww]{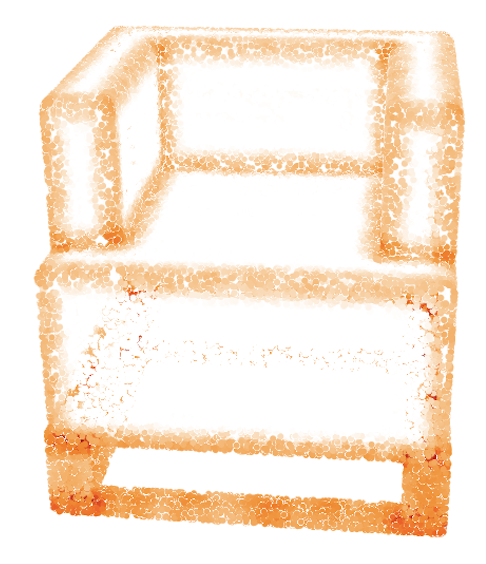}} &
\T{\includegraphics[width=\imww]{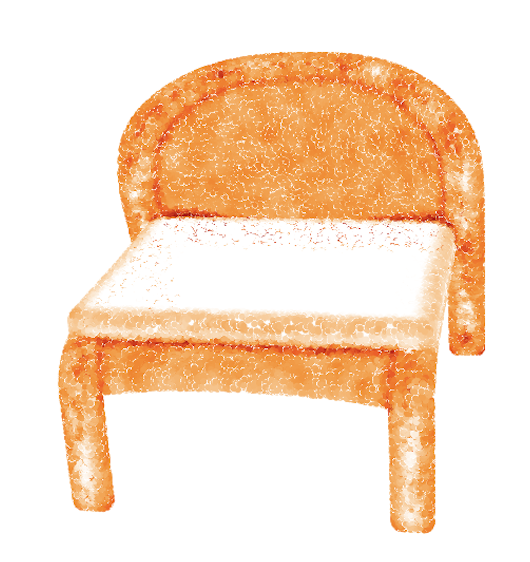}} &
\T{\includegraphics[width=\imww]{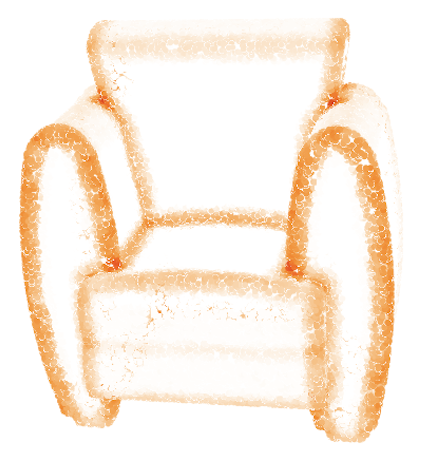}} &
\T{\includegraphics[width=\imww] {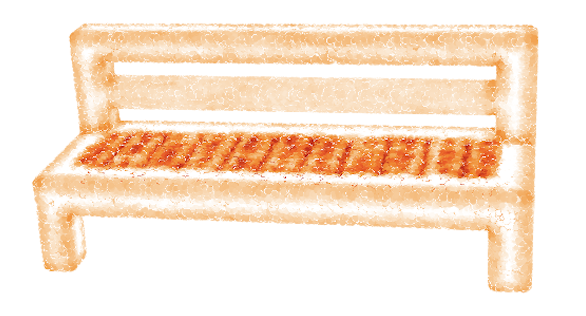}} &
%\T{\includegraphics[width=\imw] {Images/sv_vis/airplane5.png}} &
\T{\includegraphics[width=\imww] {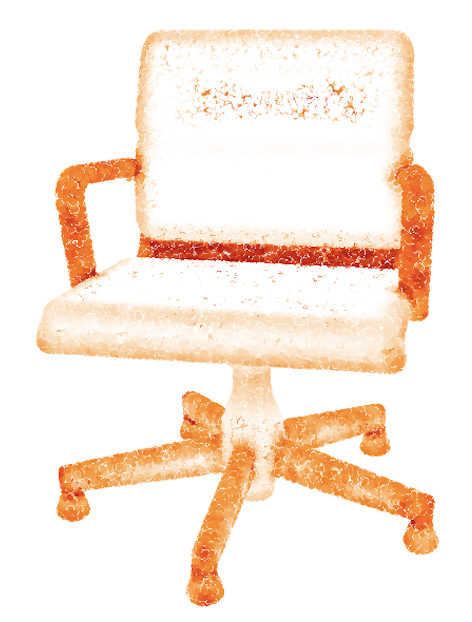}} 
\\ 
\T{\includegraphics[width=\imww]{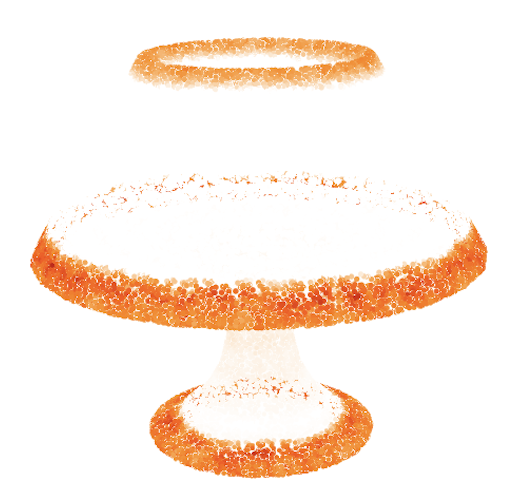}} &
\T{\includegraphics[width=\imww]{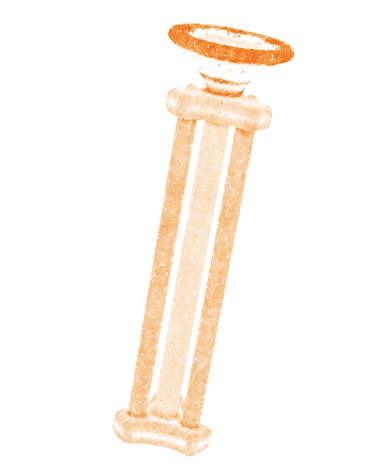}} &
\T{\includegraphics[width=\imww]{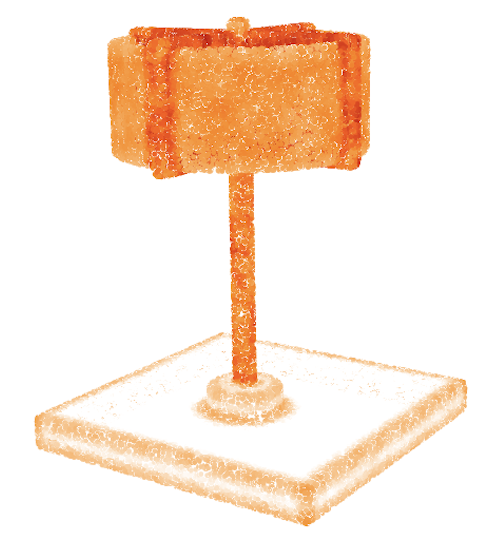}} &
\T{\includegraphics[width=\imww]{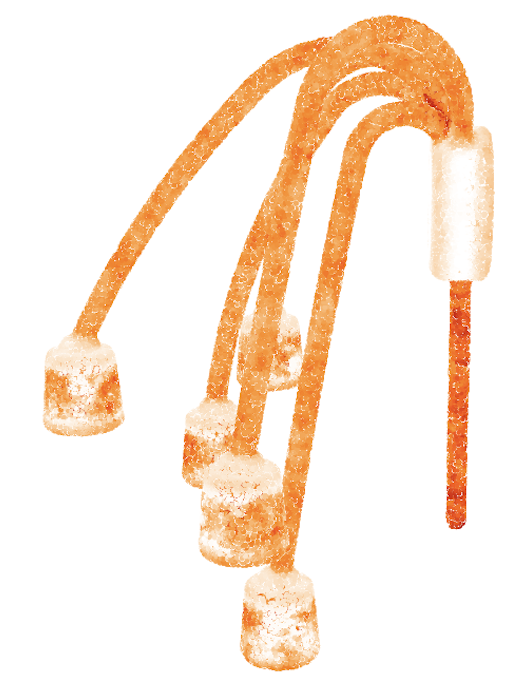}} &
\T{\includegraphics[width=\imww] {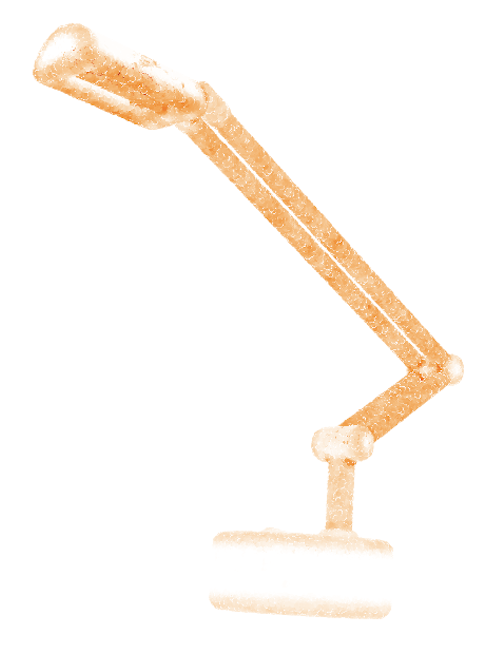}} &
\T{\includegraphics[width=\imww] {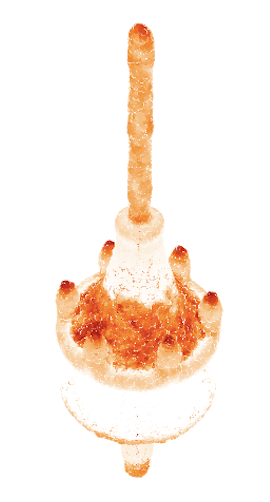}} 
\\ 
\end{tabular}

\caption{\textbf{Visualization results of shape surface variation in the ShapeNet dataset.} Red means high values and white means low values.}
%Note that the color coding is different from the main paper, we change it for better visualization.}
\label{fig:sv_vis}
\end{figure*}
