# Supplementary material for: Representation Learning for Point Cloud Understanding
Source: arXiv:2512.06058 source file (2025-12-05)
Supplement: Supplementary file 16 [file supp_ablation.tex]

\begin{table*}[t]
%\scriptsize
\setlength\tabcolsep{10pt}
\begin{subtable}[t]{.3\textwidth}
\centering  
%\scriptsize
\footnotesize
\caption{\footnotesize \textbf{Neighborhood size}}
    \begin{tabular}{cc}
    \toprule
     r & ScanObjectNN \\
        \midrule
        0.05 & 86.6 \\
        0.07 & 87.0 \\
        \rowcolor{gray!20} 0.1 & \textbf{87.7} \\
        0.2 & 86.8 \\
        \bottomrule
    \end{tabular}
     \label{tab:sv_ablation}
\end{subtable}
 %\hfill
 \hspace*{0.017\textwidth}
\begin{subtable}[t]{.3\textwidth}
\centering  
%\scriptsize
\footnotesize
\caption{\footnotesize \textbf{Number $k$ in FPS}} 
\begin{tabular}{cc}
\toprule
        \# $k$ & ScanObjectNN \\ 
        \midrule
        8 & 87.4 \\
        16 & 87.4 \\
        \rowcolor{gray!20} 32 & \textbf{87.7} \\
        64 & 87.6 \\
        128 & 87.6 \\
        \bottomrule
    \end{tabular}
    \label{tab:fps}
\end{subtable}
 %\hfill 
\begin{subtable}[t]{.33\textwidth}
\centering  
\footnotesize
\caption{\footnotesize \textbf{Mask region}} 
    \begin{tabular}{cc}
    \toprule
     region & ScanObjectNN \\
        \midrule
        \rowcolor{gray!20} masked only & \textbf{87.7} \\
        all points & 86.8 \\
        \bottomrule
    \end{tabular}
    \label{tab:unmasked}
\end{subtable}

\caption{\small{\textbf{More ablation studies of our design choices}. Please refer to \cref{sec:supp-ablation} for more details.}}
\label{tab:ablation} \vspace{-5mm}
\end{table*}
