# Supplementary material for: Representation Learning for Point Cloud Understanding
Source: arXiv:2512.06058 source file (2025-12-05)
Supplement: Supplementary file 17 [file supp_fps.tex]

\begin{table}[h]
    \centering
    %\footnotesize
    \vspace{-7pt}
    \scriptsize
    \begin{tabular}{cccccc}
        %\toprule
        \# $k$ & 8 & 16 & 32 & 64 & 128 \\
        \midrule
        ScanObjectNN & 87.4 & 87.4 & \textbf{87.7} & 87.6 & 87.6 \\
        %\bottomrule
    \end{tabular}
    %\caption{}
    \vspace{-12pt}
    \label{tab:fps} 
\end{table}
