# Supplementary material for: Representation Learning for Point Cloud Understanding
Source: arXiv:2512.06058 source file (2025-12-05)
Supplement: Supplementary file 18 [file supp_unmasked.tex]

\begin{table}[h]
    \centering
    \scriptsize
    %\footnotesize
    \vspace{-8pt}
    \begin{tabular}{ccc}
        %\toprule
         & \textbf{masked only} & \textbf{all points} \\
        \midrule
        ScanObjectNN (PB-T50-RS) & \textbf{87.7} & 86.8 \\
        %\bottomrule
    \end{tabular}
    %\caption{}
    \vspace{-12pt}
    \label{tab:supp-unmask}
    
\end{table}
